# Supplementary material for: BERT Rankers are Brittle: a Study using Adversarial Document Perturbations
Source: arXiv:2206.11724 source file (2022-06-23)
Supplement: Supplementary file 1 [file appendix.tex]

\begin{figure}[t!]
      \centering
      \includegraphics[width=0.9\linewidth]{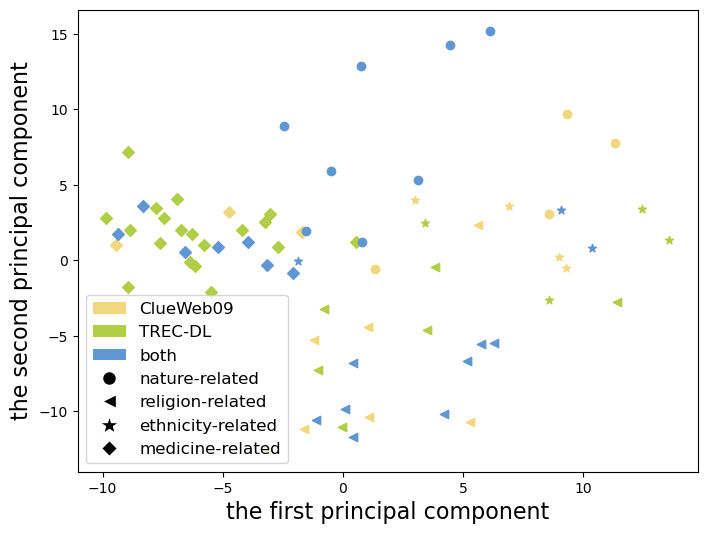}
      \caption{Frequently appeared adversary tokens from instance-wise attacking for both datasets. Note that the topic of each token is manually assigned. }
      \label{fig:pca}
    \end{figure}

\begin{figure}[t!]
      \centering
      \includegraphics[width=0.9\linewidth]{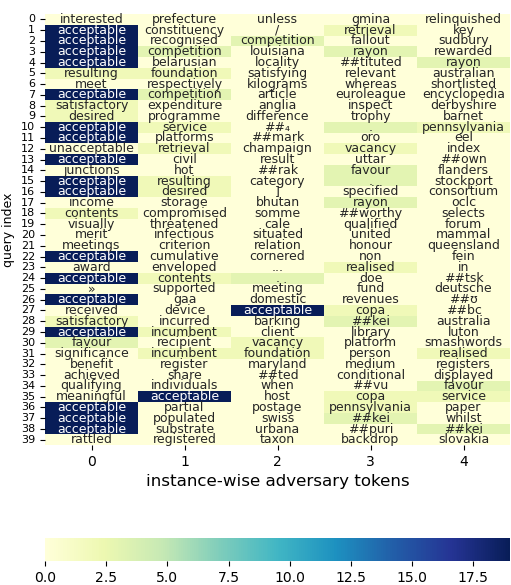}
      \caption{Adversarial tokens from instance-wise attacking for ClueWeb09 document demotion. Specific tokens frequently occurred across queries.}
      \label{fig:heatmap}
    \end{figure}
    
\begin{figure}[t!]
      \centering
      \includegraphics[width=0.8\linewidth]{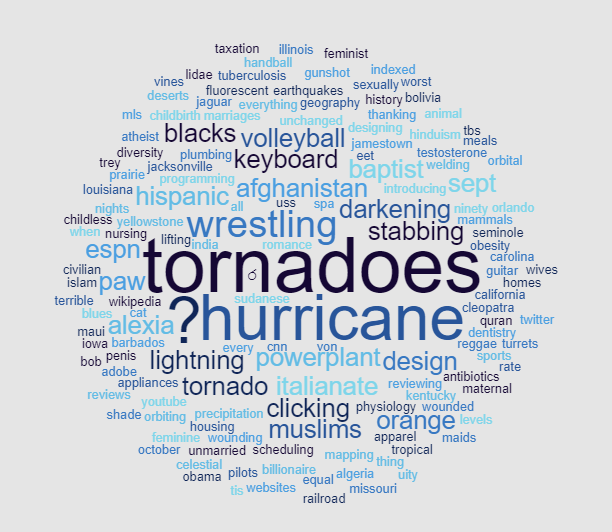}
      \caption{Adversarial tokens from instance-wise attacking for ClueWeb09 document promotion. Tokens related to natural disaster are frequently occurred across queries. }
      \label{fig:wordcloud}
    \end{figure}
